# Supplementary material for: Maximum Matching in Two, Three, and a Few More Passes Over Graph Streams
Source: arXiv:1702.02559 source file (2017-04-21)
Supplement: Supplementary file 1 [file appendix.tex]

%%% Local Variables:
%%% mode: latex
%%% TeX-master: "main_twopass"
%%% End:
